# Supplementary material for: Electronic Structure of ThPd$_2$Al$_3$: an impact of the U $5f$ states in the electronic structure of UPd$_2$Al$_3$
Source: arXiv:2203.03790 source file (2022-03-08)
Supplement: Supplementary file 1 [file ThPd2Al3_suppl.pdf]

# Supplementary Materials for Electronic structure of $ThPd_2Al_3$: an impact of the U 5$f$ states in the electronic structure of $UPd_2Al_3$

Shin-ichi Fujimori,[1] Yukiharu Takeda,[1] Hiroshi Yamagami,[1,2]
Jiří Pospíšil,[3,4] Etsuji Yamamoto,[3] and Yoshinori Haga[3]

[1]Materials Sciences Research Center,
Japan Atomic Energy Agency, Sayo, Hyogo 679-5148, Japan

[2]Department of Physics, Faculty of Science,
Kyoto Sangyo University, Kyoto 603-8555, Japan

[3]Advanced Science Research Center,
Japan Atomic Energy Agency, Tokai, Ibaraki 319-1195, Japan

[4]Department of Condensed Matter Physics,
Faculty of Mathematics and Physics, Charles University,
Ke Karlovu 5, 121 16 Prague 2, Czech Republic

## I. OVERVIEW OF BAND-STRUCTURE CALCULATION

In the present study, we have employed all-electron fully-relativistic spin-polarized self-consistent band-structure calculations with the linearized-argumented-plane-wave (LAPW) method [1] based on the local density approximation (LDA)[2]. In this approach, the usual LAPW method [3] is generalized by the Dirac-type Kohn-Sham equation, and all relativistic effects, including spin-orbit interaction, are taken into account a priori. Here it is relevant to mention that this extension has been carried out in many other band theories, as detailed in the introduction of the paper [4] for the linear augmented-Slater-type-orbital method.

To solve a band-energy $E_\lambda(\boldsymbol{k})$ and the corresponding Bloch function $\Phi_\lambda(\boldsymbol{k}, r)$ with a band-index $\lambda$ and a reduced wave vector $\boldsymbol{k}$ in the Brillouin zone, the Dirac-type Kohn-Sham equation is assumed as follows;

$$\hat{H}\Phi_\lambda(\boldsymbol{k}, \boldsymbol{r}) = E(\boldsymbol{k})\Phi_\lambda(\boldsymbol{k}, \boldsymbol{r}) \quad , \tag{1}$$

where

$$\hat{H} = c\alpha \cdot \boldsymbol{p} + (\beta - I)m_0c^2 + V(\boldsymbol{r}) + \beta\sigma_z B(\boldsymbol{r}) \quad , \tag{2}$$

where $c$, $m_0$, and $\boldsymbol{p}$ are the light velocity, the rest-mass of electron, and the momentum operator, respectively. The operators $\alpha$, $\beta$, and $I$ denote the standard Dirac $4 \times 4$ matrices [5], and $\sigma_z$ is the $z$-component of the Pauli matrix. The effective scalar-potential $V(\boldsymbol{r})$ and the magnetic-field $B(\boldsymbol{r})$ along the $z$ axis are expressed as follows;

$$V(\boldsymbol{r}) = V_{\text{ext}}(\boldsymbol{r}) + e^2 \int_\Omega d\boldsymbol{r}' \frac{n(\boldsymbol{r}')}{|\boldsymbol{r} - \boldsymbol{r}'|} + \frac{\delta E_{\text{XC}}[n(\boldsymbol{r}), m(\boldsymbol{r})]}{\delta n(\boldsymbol{r})} \quad , \tag{3}$$

and

$$B(\boldsymbol{r}) = B_{\text{ext}}(\boldsymbol{r}) + \frac{\delta E_{\text{XC}}[n(\boldsymbol{r}), m(\boldsymbol{r})]}{\delta m(\boldsymbol{r})} \quad , \tag{4}$$

where $E_{\text{XC}}$ is an exchange-correlation energy in a local-density approximation [2]. Then, $n(\boldsymbol{r})$ and $m(\boldsymbol{r})$ are the charge density and the spin-magnetization density, respectively, as expressed following;

$$n(\boldsymbol{r}) = \sum_{\lambda, \boldsymbol{k}} \Phi_\lambda^\dagger(\boldsymbol{k}, \boldsymbol{r})\Phi_\lambda(\boldsymbol{k}, \boldsymbol{r})\theta(E_{\text{F}} - E_\lambda(\boldsymbol{k})) \quad , \tag{5}$$

and

$$m(\boldsymbol{r}) = \sum_{\lambda, \boldsymbol{k}} \Phi_\lambda^\dagger(\boldsymbol{k}, \boldsymbol{r})\beta\sigma_z\Phi_\lambda(\boldsymbol{k}, \boldsymbol{r})\theta(E_{\text{F}} - E_\lambda(\boldsymbol{k})) \quad , \tag{6}$$

where $\theta(x)$ and $E_{\mathrm{F}}$ represent the step function and the Fermi energy, respectively. The Bloch wave function $\Phi_\lambda(\boldsymbol{k},\boldsymbol{r})$ is expressed by basis functions $\Psi(\boldsymbol{k}_j,m;\boldsymbol{r})$;

$$\Phi_\lambda(\boldsymbol{k},\boldsymbol{r}) = \frac{1}{\sqrt{\Omega}}\sum_j \sum_{m=\pm\frac{1}{2}} U_\lambda(\boldsymbol{k}_j,m)\Psi(\boldsymbol{k}_j,m;\boldsymbol{r}) \quad , \tag{7}$$

where $\boldsymbol{\Omega}$ is the volume of the unit cell, and $\boldsymbol{k}_j$ is defined by the reciprocal lattice vector $\boldsymbol{K}_j$ as $\boldsymbol{k}_j = \boldsymbol{k} + \boldsymbol{K}_j$.

In the family of (L)APW methods, the unit cell is usually divided into two types of regions: One is the APW region, which is the space inside the APW spheres surrounding the nucleus, and the other is the intermediate region outside the APW spheres. In the interstitial region, the basis function for (7) is defined by the relativistic plane wave function [6];

$$\Psi_{\mathrm{o}}(\boldsymbol{k},m;\boldsymbol{r}) = \sqrt{\frac{k^0+m_0c^2}{2k^0}}\begin{pmatrix} \chi(m) \\ \frac{\hbar c\sigma\cdot\boldsymbol{k}}{k^0+m_0c^2}\chi(m)\end{pmatrix}\exp(i\boldsymbol{k}\cdot\boldsymbol{r}) \quad , \tag{8}$$

where $\chi(m)$ is the spinor function with respect to the spin state $m=\pm\frac{1}{2}$ and $k^0$ denotes the relativistic energy associated with the wave vector $\boldsymbol{k}$ as,

$$k^0 = c\sqrt{(\hbar k)^2 + (m_0c^2)^2} \quad . \tag{9}$$

In the APW region, the spherically-expanded functions are utilized as the basis function: Suppose that a given solid is composed of group-theoretically independent kinds of atoms $n_a$. The basis function inside the APW sphere of radius $a_p$ at the $\nu$th atom belonging to the $p$th kind of $n_a$, which is located by the position vector $\boldsymbol{t}_\nu^p$, is represented using a vector $\boldsymbol{r}_\nu^p = \boldsymbol{r} - \boldsymbol{t}_\nu^p$ as follows;

$$\begin{aligned}\Psi_i(\boldsymbol{k},m;\boldsymbol{r}) = \exp(i\boldsymbol{k}\cdot\boldsymbol{t}_\nu^p)\sqrt{\frac{k^0+m_0c^2}{2k^0}}\sum_l \sqrt{4\pi}i^\ell a_p \\ \times\sum_\mu \sum_{\alpha=\pm\frac{1}{2}}\left(B_{\ell\mu}^{\alpha p}(\boldsymbol{k},m)\psi_{\ell\mu}^{\alpha p}(\boldsymbol{r}_\mu^p) + \dot{B}_{\ell\mu}^{\alpha p}(\boldsymbol{k},m)\dot{\psi}_{\ell\mu}^{\alpha p}(\boldsymbol{r}_\mu^p)\right) \quad ,\end{aligned} \tag{10}$$

where the wave function $\psi_{\ell\mu}^{\alpha p}(\boldsymbol{r})$ with $\alpha=\pm\frac{1}{2}$ is expressed as

$$\psi_{\ell\mu}^{\alpha p}(\boldsymbol{r}) = \frac{1}{r}\sum_{s=\pm\frac{1}{2}}\begin{pmatrix} g_s^{\ell\mu;\alpha p}(r)\chi_s^{\ell;\mu}(\hat{r}) \\ if_s^{\ell\mu;\alpha p}(r)\chi_{-s}^{\ell+2s;\mu}(\hat{r})\end{pmatrix} \tag{11}$$

and the corresponding energy-derivative function, $\dot{\psi}_{\ell\mu}^{\alpha p}(\boldsymbol{r}_\mu^p) = \partial\psi_{\ell\mu}^{\alpha p}(\boldsymbol{r}_\mu^p)/\partial\varepsilon$ [7]. Then $\chi_s^{\ell;\mu}(\hat{r})$ is the normalized spin-angular function [5, 6], which is formed by a linear combination of the

Pauli spinor and the spherical harmonics $Y_\ell^{\mu-m}(\hat{r})$ of order $\ell$ as

$$\chi_s^{\ell;\mu}(\hat{r}) = \sum_{m=\pm\frac{1}{2}} C_{sm}^{\ell;\mu} Y_\ell^{\mu-m}(\hat{r})\,\chi(m) \quad , \tag{12}$$

where the coefficients $C_{sm}^{\ell;\mu}$ denote the Clebsch-Gordan (CG) coefficient, defined by the matrices $\boldsymbol{C}^{\ell\mu}$

$$\begin{aligned} C^{\ell;\mu} &= \begin{pmatrix} C_{\frac{1}{2}\frac{1}{2}}^{\ell;\mu} & C_{\frac{1}{2}-\frac{1}{2}}^{\ell;\mu} \\ C_{-\frac{1}{2}\frac{1}{2}}^{\ell;\mu} & C_{-\frac{1}{2}-\frac{1}{2}}^{\ell;\mu} \end{pmatrix} \\ &= \frac{1}{\sqrt{2}} \begin{pmatrix} \sqrt{1+u_\mu^\ell} & \sqrt{1-u_\mu^\ell} \\ -\sqrt{1-u_\mu^\ell} & \sqrt{1+u_\mu^\ell} \end{pmatrix} \end{aligned} \tag{13}$$

with the parameter

$$u_\mu^\ell = \frac{\mu}{\ell+\frac{1}{2}} \quad . \tag{14}$$

For paramagnets at $B(\boldsymbol{r}) = 0$, the radial functions $g_s^{\ell\mu;\alpha p}(r)$ and $f_s^{\ell\mu;\alpha p}(r)$ in eq. (11) are diagonalized to $\alpha = s$ and correspond exactly to the small and large components of the Dirac radial wave function, respectively [5], while for magnets, the radial functions with $\alpha$ are coupled on the order of $c^{-2}$ for the two states of $j = \ell + s$ with $s = \pm\frac{1}{2}$ except $\ell = 0$. For a fixed energy $\epsilon_{\ell\mu}^{\alpha p}$, the simultaneous differential equations for the radial functions are derived from $\hat{H}\psi_{\ell\mu}^{\alpha p}(\boldsymbol{r}) = \epsilon_{\ell\mu}^{\alpha p}\psi_{\ell\mu}^{\alpha p}(\boldsymbol{r})$ as follows,

$$\left(\frac{\mathrm{d}}{\mathrm{dr}} + \frac{\kappa_s^\ell}{r}\right) g_s^{\ell\mu;\alpha p}(r) \; - \; \left[1 + \frac{1}{c^2}(\epsilon_{\ell\mu}^{\alpha p} - V^p(r) - 2sB^p(r)u_\mu^{\ell+2s})\right] c f_s^{\ell\mu;\alpha p}(r) = 0 \quad , \tag{15}$$

$$\begin{aligned} \left(\frac{\mathrm{d}}{\mathrm{dr}} - \frac{\kappa_s^\ell}{r}\right) c f_s^{\ell\mu;\alpha p}(r) \; &+ \; \left(\epsilon_{\ell\mu}^{\alpha p} - V^p(r) - 2sB^p(r)u_\mu^\ell\right) g_s^{\ell\mu;\alpha p}(r) \\ &+ \; B^p(r)\sqrt{1-(u_\mu^\ell)^2}\, g_{-s}^{\ell\mu;\alpha p}(r) = 0 \quad , \end{aligned} \tag{16}$$

using $\kappa_s^\ell = -2s(\ell + s + \frac{1}{2})$ for $s = \pm\frac{1}{2}$, where $V^p(r)$ and $B^p(r)$ represent the effective scalar-potential and the magnetic-field in the APW sphere of the $p$th kind, respectively. The above four differential equations for $s = \pm\frac{1}{2}$ are called spin-polarized coupled Dirac equations, and their numerical solutions are described in detail elsewhere [8]. Similarly, the radial functions of the energy-derivative function, $\dot{\psi}_{\ell\mu}^{\alpha p}(\boldsymbol{r}_\mu^p)$, are derived from $\hat{H}\dot{\psi}_{\ell\mu}^{\alpha p}(\boldsymbol{r}) = \epsilon_{\ell\mu}^{\alpha p}\dot{\psi}_{\ell\mu}^{\alpha p}(\boldsymbol{r}) + \psi_{\ell\mu}^{\alpha p}(\boldsymbol{r})$ [1, 4], although the equations are not given in detail here. Moreover, the expansion coefficients $B_{\ell\mu}^{\alpha p}(\boldsymbol{k}, m)$ and $\dot{B}_{\ell\mu}^{\alpha p}(\boldsymbol{k}, m)$ in Eq. (11) are determined from the condition that

the intermediate basis functions (8) and the APW basis functions (10) are continuously connected on the APW sphere of the $p$th kind [1].

Finally, the band-energy $E_\lambda(\boldsymbol{k})$ and the corresponding eigenvectors $U_\lambda(\boldsymbol{k}_j, m)$ are obtained by solving the set of equation,

$$\sum_j \sum_n \left[ H_{ij}^{mn} - E_\lambda(\boldsymbol{k}) O_{ij}^{mn} \right] U_\lambda(\boldsymbol{k}_j, n) = 0 \quad , \tag{17}$$

with the Hamiltonian matrix elements

$$H_{ij}^{mn} = \frac{1}{\Omega} \int_\Omega \mathrm{d}\boldsymbol{r} \Psi^\dagger(\boldsymbol{k}_i, m; \boldsymbol{r}) \; \hat{H} \; \Psi(\boldsymbol{k}_j, n; \boldsymbol{r}) \quad , \tag{18}$$

and the overlapping matrix elements

$$O_{ij}^{mn} = \frac{1}{\Omega} \int_\Omega \mathrm{d}\boldsymbol{r} \Psi^\dagger(\boldsymbol{k}_i, m; \boldsymbol{r}) \Psi(\boldsymbol{k}_j, n; \boldsymbol{r}) \quad . \tag{19}$$

In the present self-consistent calculations, the $5f$, $6p$, $6d$, and $7s$ states of U and Th atoms are treated as valence electrons, and $5s$ and other states are treated as core states within their APW spheres. For any solid, the basis function in the APW region are expanded up to $\ell = 8$. As for the lattice constants, experimental values were used, and the radius of the APW sphere $a_p$ was set to be the largest value unless they overlap. Then the number of relativistic plane waves in the intermediate region should be about 400 for $ThPd_2Al_3$ to achieve enough convergence for the band dispersion. In obtaining the charge density (5) and the spin-magnetization density (6), the sums over the occupied states are perform with the tetrahedron method[9], and the sampling $\boldsymbol{k}$-points are generalized up to 726 points in the irreducible wadge of hexagonal Brillouin zone.

[1] H. Yamagami, All-Electron Spin-Polarized Relativistic Linearized APW Method: Electronic and Magnetic Properties of BCC Fe, HCP Gd and Uranium Monochalcogenides, J. Phys. Soc. Jpn. 67, 3176 (1998).

[2] U. von Barth and L. Hedin, A local exchange-correlation potential for the spin polarized case. i, J. Phys. C: Solid State Phys. 5, 1629 (1972).

[3] D. J. Singh and J. Nordström, Planewave, Psuedopotentials and The LAPW Method 2nd edn (Berlin: Springer, 2006).

[4] H. Yamagami and Y. Kitawaki, Spin-polarized relativistic calculations in linear augmented-slater-type-orbital method, Electron. Struct. 3, 034003 (2021).

[5] J. J. Sakurai, Adovanced Quantum Mechanics (Addison-Wesley, 1967).

[6] T. L. Loucks, Augmented plane wave method: a guide to performing electronic structure calculations, 28 (WA Benjamin, 1967).

[7] O. K. Andersen, Linear methods in band theory, Phys. Rev. B 12, 3060 (1975).

[8] H. Yamagami, A. Mavromaras, and J. Kübler, Magnetic properties of f-electron systems in spin-polarized relativistic density functional theory, Journal of Physics: Condensed Matter 9, 10881 (1997).

[9] P. E. Blöckl, O. Jepson, and O. K. Anderson, Improved tetrahedron method for Brillouin-zone integrations, Phys. Rev. B 49, 16223 (1994).
